# Supplementary material for: Inferring the Isotropic-nematic Phase Transition with Generative Machine Learning
Source: arXiv:2410.21034 source file (2024-10-28)
Supplement: Supplementary file 1 [file SI.pdf]

# Supplementary Information for: Inferring the Isotropic-nematic Phase Transition with Generative Machine Learning

Eric R. Beyerle and Pratyush Tiwary

August 2024

## 1 Parameterization of the Gay-Berne Potential

The simulations of the Gay-Berne melts presented in the main text are performed using LAMMPS, with the potential given in Ref. [1]. Precisely, we invoke the `pair_style gayberne` directive in the LAMMPS script used to run the simulations. Specifically, the Gay-Berne potential is defined using the following lines in the LAMMPS input file:

```
pair_style gayberne 1.0 1.0 2.0 4.0
pair_coeff 1 1 1.0 1.0 1 1 0.2 1 1 0.2
pair_modify shift yes
```

These instructions define a Gay-Berne potential as given in Ref. [1] with  $\gamma = 1.0$ ,  $v = 1.0$ ,  $\mu = 2.0$ , and a cutoff distance of  $4.0\sigma$  with the potential shifted to zero at the cutoff. Furthermore, the `pair_modify` directive defines a well depth of  $1.0\epsilon$ , a minimum effective particle radius of  $1.0\sigma$ , side-side interaction well depths of  $1.0\epsilon$ , and end-end interaction well depths of  $0.2\epsilon$ . LAMMPS input files for the equilibration and production simulations are given in the associated GitHub repository [2].

In practice, the GB potential is implemented in LAMMPS as follows, which follows closely the LAMMPS documentation. [3] The pairwise interaction of the GB ellipsoids is evaluated as a product of three terms:

$$U(\mathbf{A}_1, \mathbf{A}_2, \mathbf{r}_{12}) = \mathbf{U}_r(\mathbf{A}_1, \mathbf{A}_2, \mathbf{r}_{12}, \gamma) \cdot \eta_{12}(\mathbf{A}_1, \mathbf{A}_2, v) \cdot \chi_{12}(\mathbf{A}_1, \mathbf{A}_2, \mathbf{r}_{12}, \mu), \quad (1)$$

where  $\mathbf{A}_i$  describes the rotation from the lab frame of reference to the particle  $i$  frame of reference,  $\mathbf{r}_{ij}$  is the center-to-center distance vector between particles  $i$  and  $j$ ; finally,  $\gamma$ ,  $v$ , and  $\mu$  are parameters. The parameter  $\gamma$  controls the shift of the minimum of the Lennard-Jones interaction between particles as follows:

$$U_r = 4\epsilon (\varrho^{12} - \varrho^6) \quad (2)$$

$$\varrho = \frac{\sigma}{h_{12} + \gamma\sigma}, \quad (3)$$

where  $h_{ij}$  is the distance of closest approach of ellipsoids  $i$  and  $j$ . Meanwhile,  $v$  determines the form of the second term as follows:

$$\eta_{12}(\mathbf{A}_1, \mathbf{A}_2, v) = \left[ \frac{2s_1s_2}{\det[\mathbf{G}_{12}(\mathbf{A}_1, \mathbf{A}_2)]} \right]^{v/2} \quad (4)$$

$$s_i = [a_ib_i + c_ic_i] [a_ib_i]^{1/2}. \quad (5)$$

In eq. 5,  $a_i$ ,  $b_i$ , and  $c_i$  refer to the three ellipsoid radii; in practice, since we simulate uniaxial GB ellipsoids here,  $b_i = c_i$ . Furthermore,

$$\mathbf{G}_{12} = \mathbf{A}_1^T \mathbf{S}_1^2 \mathbf{A}_1 + \mathbf{A}_2^T \mathbf{S}_2^2 \mathbf{A}_2, \quad (6)$$

with  $\mathbf{S}_i = \text{diag}(a_i, b_i, c_i)$ ; eq. 6 gives the relative orientations between two particles in the body-fixed frame of reference.

Finally,  $\mu$  controls the form of the third term in the potential:

$$\chi_{12} = [2\hat{\mathbf{r}}_{12}\mathbf{B}_{12}^{-1}\hat{\mathbf{r}}_{12}]^\mu, \quad (7)$$

with  $\hat{\mathbf{r}}_{ij} = \mathbf{r}_{ij}/|\mathbf{r}_{ij}|$  and

$$\mathbf{B}_{ij} = \mathbf{A}_i^T \mathbf{E}_i \mathbf{A}_i + \mathbf{A}_j^T \mathbf{E}_j \mathbf{A}_j, \quad (8)$$

with  $\mathbf{E}_i = \text{diag}(\epsilon_{ia}^{-1/\mu}, \epsilon_{ib}^{-1/\mu}, \epsilon_{ic}^{-1/\mu})$  is the diagonal matrix storing the anisotropic interactions for particle  $i$ . Finally, the distance of closest approach is approximated using the Perram reference [4]:

$$h_{12} = r - \sigma_{12}(\mathbf{A}_1, \mathbf{A}_2, \mathbf{r}_{12})$$

with  $r = |\mathbf{r}_{12}|$  and  $\sigma_{12} = [\frac{1}{2}\hat{\mathbf{r}}_{12}^T \mathbf{G}_{12}^{-1} \hat{\mathbf{r}}_{12}]^{-1/2}$ . Details regarding the calculations of the forces and torques on the GB ellipsoids are given in the LAMMPS documentation [3] and the associated manuscript. [1]

## 2 Thermodynamic Maps Architecture, Training, and Parameterization

The score in TM is learned by minimizing the following loss function:

$$\mathcal{L} = \mathbb{E}_{\mathbf{s}_0} \mathbb{E}_{t \sim \mathcal{U}(0, T)} [\|\mathbf{u}_0 - f_\theta(\mathbf{u}_n, t)\|]. \quad (9)$$

The double expectation value  $\mathbb{E}_{\mathbf{s}_0} \mathbb{E}_{t \sim \mathcal{U}(0, T)} [\dots]$  amounts to taking a mean-squared error between the reference and inferred values of input features over the true samples ( $\mathbf{u}_0 \sim \mathbf{s}_0$ ) and inferred, denoised samples  $f_\theta(\mathbf{u}_n, t), t \sim \mathcal{U}(0, T)$ . In eq. 9,  $\mathbf{u}_n := (\mathbf{x}_n, \boldsymbol{\beta}_n^{-1})^T$  is a sample at step  $n$  of the noising process. This loss function seeks to minimize the Manhattan norm between the true and learned noise schedules. The double expectation  $\mathbb{E}_{\mathbf{s}_0} \mathbb{E}_{t \sim \mathcal{U}(0, T)} [\dots]$  is calculated over batches of the simulation data, corresponding to an empirical expectation over the training data.

The thermodynamic maps algorithm is trained using 9000 frames of the ellipsoid orientations from the molecular dynamics simulations performed at  $T^* = 1.0$  and  $T^* = 2.0$ . For hyperparameters, the number of noising steps is set to 100 using the variance preserving algorithm, the batch size is 512, and the learning rate is 0.01. The U-net architecture utilizes 8 Resnet block groups with four channels. Although there are 343 particles in each simulation, the target shape of the U-net is set to 320, due to the constraint that the target must be a multiple of 8. The score-matching loss is set equal to the smooth L1 loss function.

## 3 Results from PCA and VAE for Learning the Nematic Order Parameter

As a control, we evaluate the ability of a principal component analysis (PCA) and variational autoencoder (VAE) to learn the nematic order parameter, which is also the effective order parameter for this system at the phase points examined, as a function of temperature. First, we find that, given the orientations of each Gay-Berne ellipsoid as input, both methods fail to learn an informative RC as the TM method does. So, the projection of each orientation vector onto the director,  $\cos(\theta_i)$ , is given as the input features to both the PCA and VAE architectures. As a control, both the PCA and VAE architectures used for the Gay-Berne ellipsoid orientations were tested on the spin configurations of a  $10 \times 10$  two-dimensional Ising model sampled via Monte Carlo, [5] and both methods manage to learn the magnetization order parameter describing the disorder-to-order transition for the Ising model (results not shown).

The learned approximation of  $\mathcal{S}$  are given in Figures S1a and S1b for the PCA and VAE, respectively. In both cases, the learned order parameters are reported for each temperature by training either the PCA or

VAE on the orientations at *all* temperatures, then projecting the orientations at a given temperature onto the RC space using either the linear PCA transformation matrix or by passing the orientations through the nonlinear VAE encoder. The reported average values of the order parameter are given for each temperature, and the error bars are the sample standard deviation of the projections at each temperature. Explicitly, denoting  $\hat{\mathcal{S}}$  as the estimated order parameter from either PCA or the VAE,

$$\hat{\mathcal{S}}(T^*) = \frac{1}{M} \sum_{m=1}^M f(\mathbf{x}(m))$$

$$\sigma_{\hat{\mathcal{S}}}(T^*) = \sqrt{\frac{1}{M} \sum_{m=1}^M f(\mathbf{x}(m))^2 - \left( \frac{1}{M} \sum_{m=1}^M f(\mathbf{x}(m)) \right)^2},$$

where  $f(\cdot)$  is either the linear PCA transformation or the nonlinear VAE encoder and

$$\mathbf{x}(k) = (\hat{u}_1(m), \hat{u}_2(m), \dots, \hat{u}_i(m), \dots, \hat{u}_N(m))$$

is the set of ellipsoid orientations at frame  $m$  of the simulation performed at temperature  $T^*$ .

We see that PCA, a linear method, fails to learn anything regarding the phase transition. This result should be no surprise, since learning the order parameter, even from the projections, requires learning the square of the projection, which is a non-linear operation. This nonlinearity cannot be learned by the linear PCA method alone. The nonlinear VAE does better learning the RC, although the error in the calculation at each temperature is relatively large. These error bars are calculated as the standard deviation of the MD orientations at each temperature when fed through the VAE, i.e. it measures the spread in the learned RC at each sampled temperature. These uncertainties are large compared to those found for TM method, shown in Figure 2 in the main text. For the VAE, increasing the depth of the encoder did not change significantly the learned order parameter (data not shown).

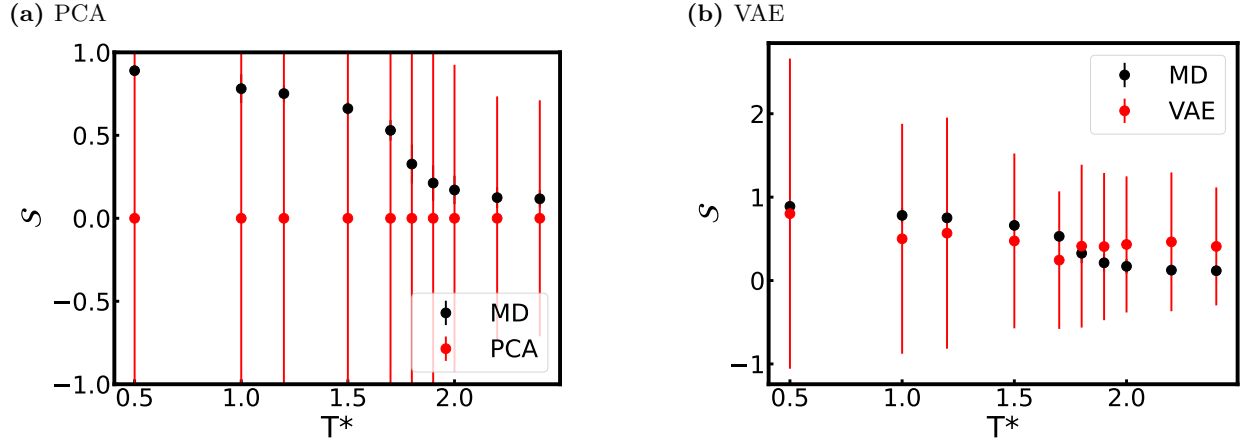

**Figure S1:** a) Reaction coordinate learned from PCA (red) as a function of reduced temperature compared to the nematic order parameter (black) calculated from the MD simulations at each temperature. b) Reaction coordinate learned from the VAE (red) as a function of reduced temperature compared to the nematic order parameter (black) calculated from the MD simulations at each temperature. The reported uncertainties are one sample standard deviation of sampled transformation of  $\cos(\theta_i)$  by the PCA or VAE encoder at each temperature.

For completeness in comparison to the TM results demonstrated in the main, we present also in Figure S2 the learned approximation of  $\mathcal{S}$  when we train the PCA and VAE on the orientations sampled at just the two temperatures,  $T^* \in \{1.0, 2.0\}$ , used to train the TM. The learned nematic order parameter  $\mathcal{S}$  is in both cases similar to the one learned when training on all the temperatures, although for the VAE, the

learned  $\mathcal{S}$  is no longer with error of 0 at low temperatures and there is a clear decreasing trend in the mean with increasing temperature. However, although the variance is still high at all temperatures. The PCA fails completely to learn anything regarding  $\mathcal{S}$ . From these results, we conclude definitively that, of the three generative models tested here, the TM approach is learning the best approximation of  $\mathcal{S}$  since it learns the mean of  $\mathcal{S}$  with a low variance at each temperature.

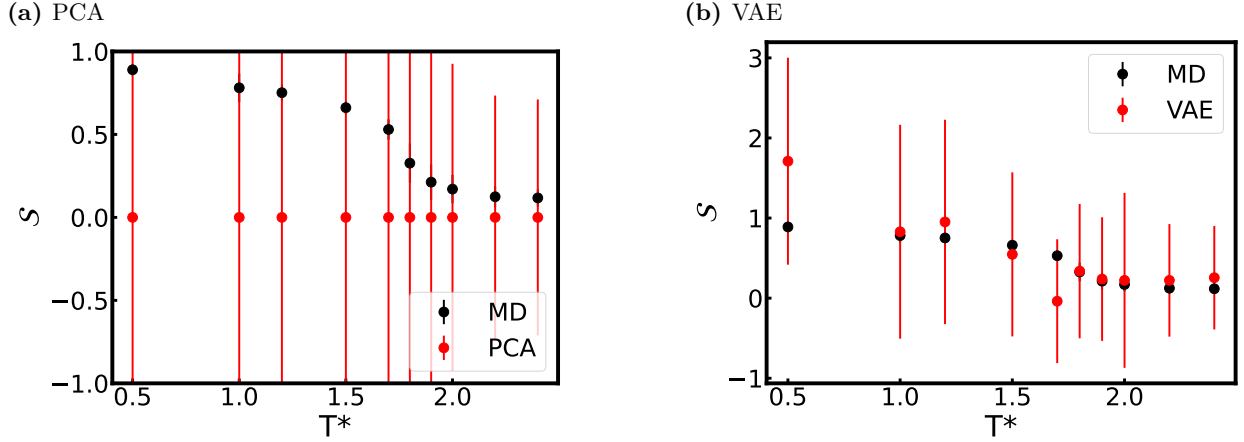

**Figure S2:** a) Reaction coordinate learned from PCA (red) as a function of reduced temperature compared to the nematic order parameter (black) calculated from the MD simulations at each temperature when trained on only the orientations sampled at  $T^* \in \{1.0, 2.0\}$ . b) Reaction coordinate learned from the VAE (red) as a function of reduced temperature compared to the nematic order parameter (black) calculated from the MD simulations at each temperature when trained on only the orientations sampled at  $T^* \in \{1.0, 2.0\}$ . The reported uncertainties are one sample standard deviation of sampled transformation of  $\cos(\theta_i)$  by the PCA or VAE encoder at each temperature. As the ordinate is limited to  $\mathcal{S} \in [-1, 1.0]$ , the full error bars are not reported.

## 4 TM versus MD Free-energy Surfaces Over All Sampled Temperatures

Figure S3 compares the free-energy in  $\mathcal{S}$  as a function of  $T^*$  over the entire sampled range of temperatures, and is simply an expansion of Figure 3 in the main text.

## 5 Power Law Fits to Heat Capacity Curves

Figure S4 shows the scaling laws fit to the heat capacity curves given in Figure 5b of the main text for both the MD and TM samples and Table S1 shows the associated scaling exponents, which are clearly within error of 0 for both the MD and TM.

**Table S1: Scaling exponents for the constant-volume heat capacity calculated using MD and TM samples fitting points both above and below the critical temperature.**

|          | MD              | TM              |
|----------|-----------------|-----------------|
| $\gamma$ | $0.0 \pm 0.1^a$ | $0.0 \pm 0.3^a$ |

<sup>a</sup>Uncertainties are reported from the curve fitting algorithm used from the Python scipy library. [6]

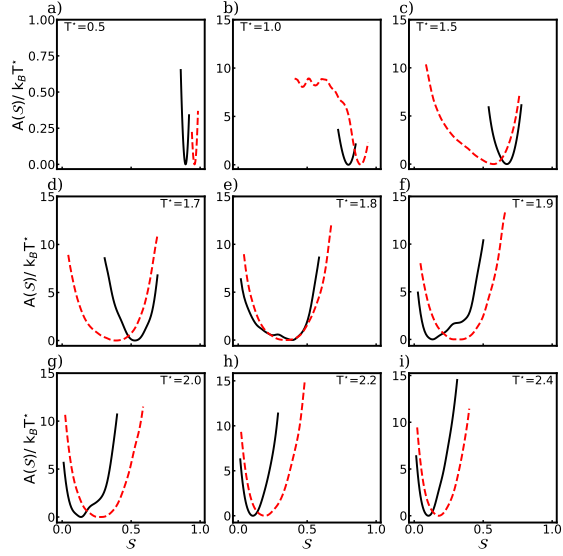

**Figure S3:** a)-i): Plots of the free-energy along the nematic order parameter  $S$  calculated from the MD (black) and TM (red, dashed) samples at the reduced temperature given in each inset. The temperature increases monotonically going left-to-right and top-to-bottom through the subplots.

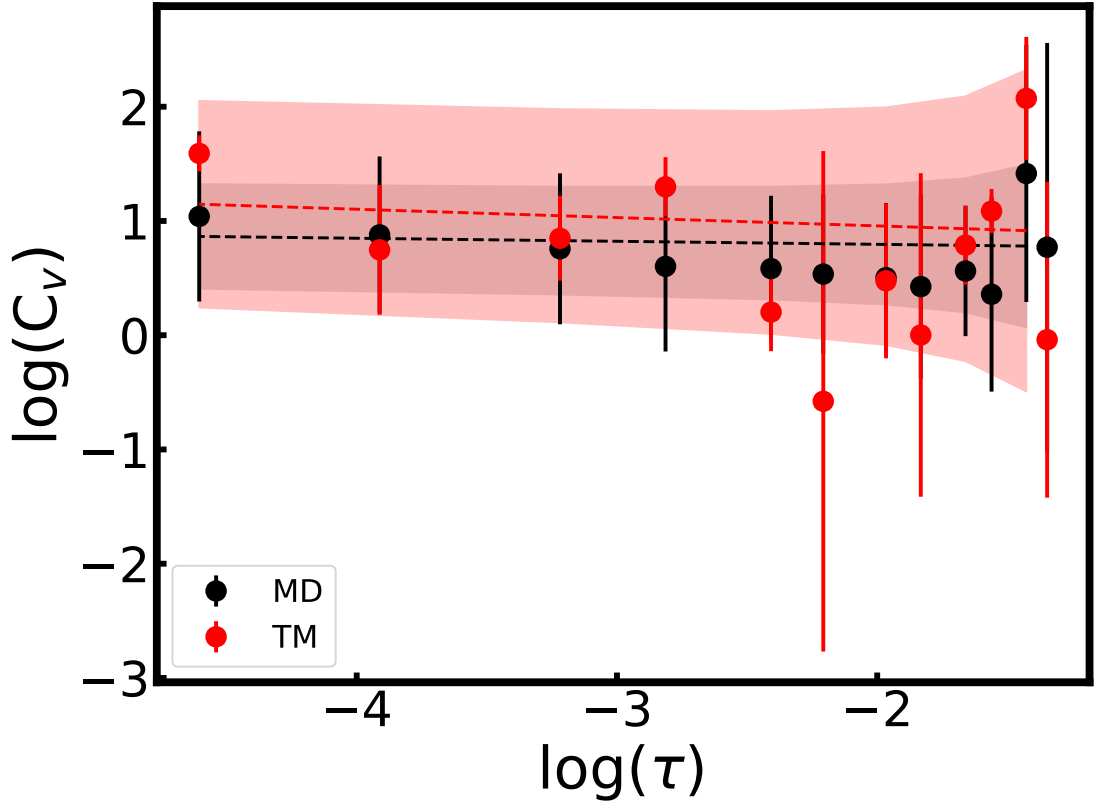

**Figure S4:** Heat capacity near the critical point calculated for the reference MD (black) and TM method (red). Power law fits are given by the dashed lines (colors the same as measured points), and the shaded regions give the uncertainties in the fit as calculated using the curve fitting algorithm in scipy. [6]

## References

- [1] W. Michael Brown, Matt K. Petersen, Steven J. Plimpton, and Gary S. Grest. Liquid crystal nanodroplets in solution. *The Journal of Chemical Physics*, 130(4):044901, 01 2009.
- [2] E. R. Beyerle. thermomaps-gayberne. <https://github.com/erb24/thermomaps-gayberne>, 2024.
- [3] Mike Brown. pair\_style gayberne command. [https://docs.lammps.org/pair\\_gayberne.html](https://docs.lammps.org/pair_gayberne.html), Jun 2024.
- [4] R. Everaers and M. R. Ejtehadi. Interaction potentials for soft and hard ellipsoids. *Physical Review E - Statistical Physics, Plasmas, Fluids, and Related Interdisciplinary Topics*, 67:8, 2003.
- [5] Lukas Herron, Kinjal Mondal, John S. Schneekloth, and Pratyush Tiwary. Inferring phase transitions and critical exponents from limited observations with Thermodynamic Maps. *arXiv e-prints*, page arXiv:2308.14885, August 2023.
- [6] Pauli Virtanen, Ralf Gommers, Travis E. Oliphant, Matt Haberland, Tyler Reddy, David Cournapeau, Evgeni Burovski, Pearu Peterson, Warren Weckesser, Jonathan Bright, Stéfan J. van der Walt, Matthew Brett, Joshua Wilson, K. Jarrod Millman, Nikolay Mayorov, Andrew R. J. Nelson, Eric Jones, Robert Kern, Eric Larson, C J Carey, İlhan Polat, Yu Feng, Eric W. Moore, Jake VanderPlas, Denis Laxalde, Josef Perktold, Robert Cimrman, Ian Henriksen, E. A. Quintero, Charles R. Harris, Anne M. Archibald, Antônio H. Ribeiro, Fabian Pedregosa, Paul van Mulbregt, and SciPy 1.0 Contributors. SciPy 1.0: Fundamental Algorithms for Scientific Computing in Python. *Nature Methods*, 17:261–272, 2020.
